# Supplementary material for: Learning the Emergent Bulk Geometry of the Three Dimensional Ising Model
Source: arXiv:2609.20210 source file (2026-07-25)
Supplement: Supplementary file 1 [file supplimentary.tex]

\documentclass[aps,prl,twocolumn,superscriptaddress,showpacs,nofootinbib]{revtex4-2}
\usepackage[colorlinks=true,linkcolor=blue,citecolor=blue]{hyperref}
\usepackage{amsmath,amssymb,amsfonts,bm}
\usepackage{graphicx}
\usepackage{xcolor}
\newcommand{\bbe}{\begin{equation}}
\newcommand{\bbq}{\end{equation}}
\newcommand{\nn}{\nonumber}
\newcommand{\ads}{\text{AdS}}
\newcommand{\Dsig}{\Delta_\sigma}
\newcommand{\Deps}{\Delta_\epsilon}
\renewcommand{\thesection}{S\arabic{section}}
\renewcommand{\theequation}{S\arabic{equation}}
\renewcommand{\thefigure}{S\arabic{figure}}
\renewcommand{\thetable}{S\arabic{table}}



\begin{document}

\title{Learning  the Emergent Bulk Geometry of the Three Dimensional Ising Model}
\author{Ritam Basu}
\email{ritam.basu@tifr.res.in}
\affiliation{Department of Theoretical Physics, Tata Institute of Fundamental
Research, 1 Homi Bhabha Road, Mumbai 400005, India}
\date{\today}
\maketitle






%% =====================================================================
\section{Monte Carlo details}

We consider the Ising model on a periodic cubic lattice of length $L$.
and coupling fixed at $\beta_c=0.2216544$\cite{Deng:2003wv,Ferrenberg:2018zst}. The single cluster algorithm of Wolff \cite{Wolff:1988uh} provides the basis for our bond update. We utilize a vectorized frontier growth search to implement the algorithm. Each bond to the current frontier is tested with the specified probability $p = 1 - e^{-2\beta}$. The algorithm tests each site independently and add aligned sites to the cluster with probability $p$. Then it flips the whole cluster. We budget a specific number of sweeps for thermalization. One complete sweep is defined by $L^3$ total spin flips. We implement this with $30$ sweeps and a completely ordered initial configuration. The ordered start speeds equilibration. Large lattices budgeted in cluster updates rather than sweeps under thermalization. A cluster update budgeted at $2000$ for $L=128$ leaves the system far from criticality, yielding $\eta_{\rm fit} \simeq 1$. The sweep budget eliminates this at all $L$. The mean cluster size at $L=128$ is observed to be $2.1 \times 10^4$ spins and is stable over the duration of the run. This stability is our equilibration diagnostic. The main analysis uses $8000$ measurements at $L=128$.  We take $8000$ measurements at $L=128$ for our main analysis.
















%% =====================================================================
\section{Momentum space observables}

The fit uses only the $k_z = 0$ plane. We therefore sum each field over the third axis before doing the Fourier transformation. This reduces the cost per measurement from a three dimensional transform to a two dimensional one.
The spin channel uses the raw field. The energy channel uses
\bbe
\varepsilon(x) = \sigma(x)\sum_\mu \sigma(x+\hat{e}_\mu) - \langle \cdot \rangle .
\bbq
The subtraction removes the mixing with the identity operator.
Momentum are those improved lattice values $\hat{k} = 2\sin(\pi n/L)$.

As a data quality check we fit the small momentum behaviour of each
channel. For the spin channel $G(k) \sim k^{-(2-\eta)}$.
For the energy channel $G_\epsilon(k) \sim k^{2\Deps - 3}$.
The measured values are collected in Table~\ref{tab:gates}.

\begin{table}[h]
\caption{Exponent checks against bootstrap values.}
\label{tab:gates}
\begin{ruledtabular}
\begin{tabular}{lccc}
$L$ & measurements & $\eta_{\rm fit}$ & $\Deps^{\rm fit}$ \\
\hline
$128$ & $8000$ & $0.069$ & $1.826$ \\
\end{tabular}
\end{ruledtabular}
\end{table}

The energy channel exponent sits above the bootstrap value of $1.4126$.
This is expected. The energy operator has strong corrections to scaling in this model. Figure~\ref{fig:scaling} shows the effective exponent drifting toward the bootstrap value as the fit window widens. Section~\ref{sec:robust} shows that the offset does not generate the tension reported in the Letter.
\begin{figure}[h]
\includegraphics[width=\linewidth]{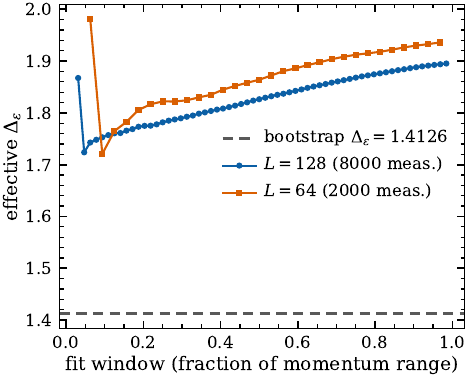}
\caption{Corrections to scaling in the energy exponent.
The effective $\Delta_\epsilon$ extracted from $G_\epsilon(k)$ is shown
against the width of the fit window, for two lattice sizes.
The dashed line is the bootstrap value. As window and lattice grows, measured exponent drifts toward it . This identifies the offset as a corrections to scaling effect rather than a defect of the data.}
\label{fig:scaling}
\end{figure}











%% =====================================================================
\section{Radial solver and quantization}
The probe equation \eqref{eq:radialS} is integrated with a fixed step
fourth-orderrth order  Runge Kutta scheme,
\bbe
\partial_z\!\Big(\frac{\sqrt{fg}}{z^2}\partial_z \phi\Big)
= \Big(\frac{\omega^2}{z^2\sqrt{fg}} + \frac{k^2 q}{z^2}
+ \frac{m^2 q}{z^4}\Big)\phi ,
\qquad q = \sqrt{f/g}.
\label{eq:radialS}
\bbq
Integration runs from an infrared wall at $z_{\rm IR} = 0.85$ to anear boundary point at $z_{\rm UV} = 0.01$.
Here we use $400$ steps. Two independent wall conditions are propagated so that the boundary data is not tied to one choice.

The coefficients $c_\pm$ in the near boundary expansion are obtained by
solving a two by two linear system at $z_{\rm UV}$ and at a second point
$z = 0.03$. All arithmetic is in double precision and this is necessary.
The exponents $\Delta_\pm$ differ by $O(1)$ and single precision loses the
sub leading coefficient.

The quantization branch is fixed per operator. Both the Ising operators have $\Delta < 3/2$ and use the alternate quantum branch, $G = c_-/c_+$. For $\Dsig = 0.5181489$ the bulk mass is $m^2 = -1.2860$ and for $\Deps = 1.412625$ it is $m^2 = -2.2424$. Both masses lie inside the window $-9/4 < m^2 < -5/4$ where the alternate quantization is admissible. The second sits just above the Breitenlohner--Freedman (BF) bound. Using the standard assignment instead produces a model correlator that grows where the data falls. We verified that the wrong assignment cannot be compensated by any geometry inside the bulk.












%% =====================================================================
\section{Gauge fixing of units}

Lattice momenta and bulk frequencies differ by a scale $s$.
Each channel also carries an overall normalization $Z$ and a contact term
$c_0$. The data is close to scale free near the critical temperature as expected. The scale $s$ is then a gauge choice, since a change of $s$ can be
absorbed into $Z$. We fix the gauge by mapping the highest measured mode to a fixed bulk frequency. $Z$ and $c_0$ are then obtained by least squares on the
ultraviolet third of the data against pure $\ads_4$ with fixed $s$.

This step is not cosmetic and without it the fit has a flat direction.
Different seeds then converge to different unit conventions and the
apparent spread in the reconstructed geometry is dominated by units rather
than by physics. With this gauge fixing the seed to seed spread in the cosmological constant falls by an order of magnitude.













%% =====================================================================
\section{Training and seed selection}

Each metric function is a two layer network with $32$ tanh-activation units. The output enters through $f = \exp(z^2 u)$ so that $f>0$ and $f \to 1$ at
the boundary. Training uses Adam with a cosine schedule and warm restarts every $700$ epochs. 

The restarts matter for the spin channel and without them the optimizer stalls on a plateau and reports a residual two orders of magnitude above the converged value.

Twenty five percent of the momentum points are held out.
They never enter the gradient of the neural network.
Early stopping keeps the snapshot with the lowest held out loss and every fit uses five seeds.

Seeds are accepted or rejected by a criterion fixed in advance.
A seed is rejected if its fitted scale drifts from the ultraviolet anchor
by more than fifty percent,
\bbe
\big| s_{\rm fit}/s_{\rm anchor} - 1 \big| > 0.5 .
\bbq
This removes runaway seeds whose unit convention has decoupled from the
data.  It removes one seed out of five values in the reported fits.
The rejected seed has a residual an order of magnitude above the others.









%% =====================================================================
\section{Resolution of the method}
\label{sec:resolution}

We calibrate on synthetic data generated from
$f = g = 1 - z^3$. The reconstruction is accurate to better than one percent for $z \lesssim 0.3$. It degrades to a few percent in the middle of the range.
and beyond $z \simeq 0.5$ the seed-to-seed band widens sharply. This behavior is intrinsic. The boundary correlator constrains the geometry through the region the probe reaches. Low-frequency modes reach deeper in the bulk.
Thus a finite momentum grid leaves the deep interior weakly determined.
We do not interpret reconstructed features beyond $z \simeq 0.3$. Also the residual comparison used in this Letter is unaffected, since it is computed at the boundary.










%% =====================================================================
\section{Robustness}
\label{sec:robust}

We repeat the full analysis under two variations. First, the
momentum window is changed by removing one further low mode. Secondly the 
lattice size is changed from $128$ to $64$. In the end we also produces data where the optimizer settings are held identical across all channels, so that the comparison is like for like.

\begin{table}[h]
\caption{Full robustness table.
Entries are medians over accepted seeds.
The fitted channel is in bold.}
\label{tab:robustfull}
\begin{ruledtabular}
\begin{tabular}{llcccc}
$L$ & cut & channel & $\mathcal{V}_\sigma$ & $\mathcal{V}_\epsilon$ & $\Lambda$ \\
\hline
128 & 2 & $\sigma$   & $\mathbf{1.9\times10^{-4}}$ & $3.6\times10^{-3}$ & $-3.24 \pm 0.42$ \\
128 & 2 & $\epsilon$ & $4.5\times10^{-2}$ & $\mathbf{9.5\times10^{-5}}$ & $-2.75 \pm 0.04$ \\
128 & 3 & $\sigma$   & $\mathbf{5.8\times10^{-4}}$ & $4.1\times10^{-3}$ & $-3.07 \pm 0.33$ \\
128 & 3 & $\epsilon$ & $2.4\times10^{-2}$ & $\mathbf{1.8\times10^{-4}}$ & $-2.81 \pm 0.03$ \\
64  & 2 & $\sigma$   & $\mathbf{8.4\times10^{-4}}$ & $3.0\times10^{-3}$ & $-3.93 \pm 1.54$ \\
64  & 2 & $\epsilon$ & $2.9\times10^{-2}$ & $\mathbf{8.2\times10^{-4}}$ & $-2.60 \pm 0.63$ \\
\end{tabular}
\end{ruledtabular}
\end{table}

Here, the predicted residual exceeds the fitted one by a factor between
$3.6$ and $4.7\times10^{2}$ across all variations.










%% =====================================================================
\section{The spin two channel}
\begin{figure}[htbp]
\includegraphics[width=0.46\textwidth]{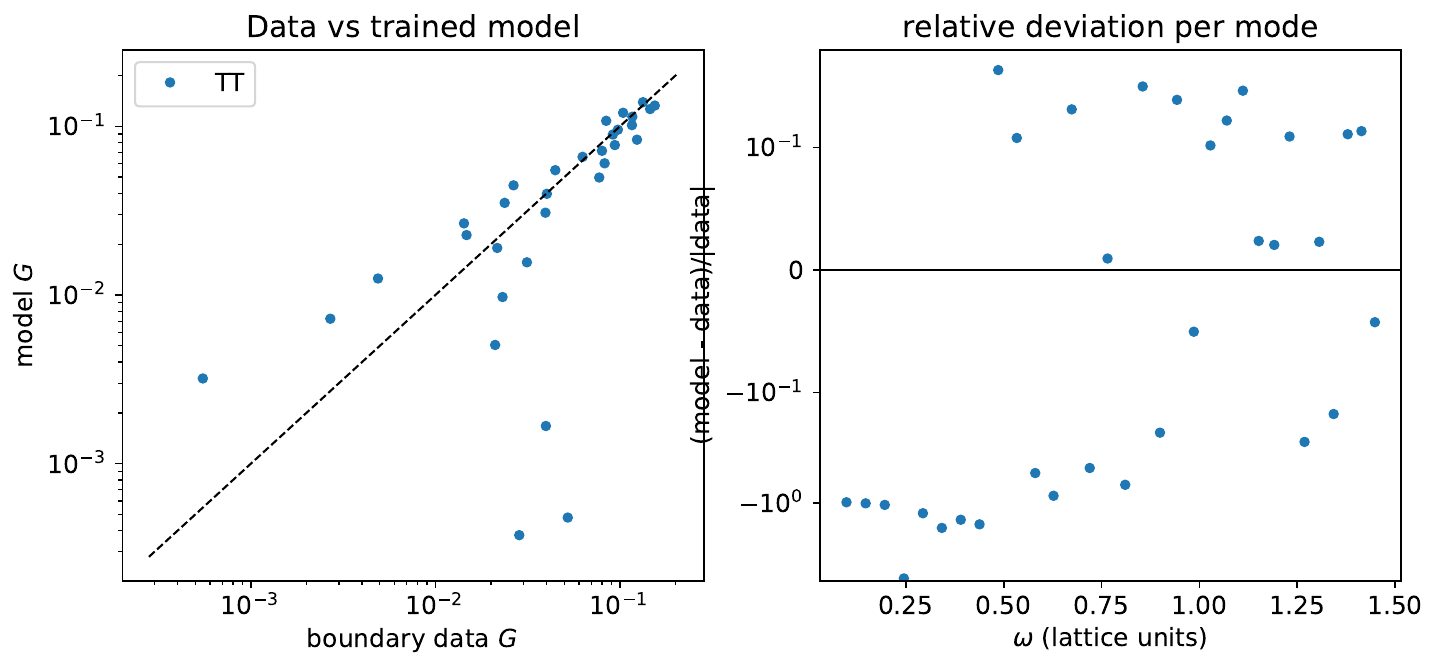}
\caption{Spin two channel.
Left, model against data.
Right, relative deviation per mode.
The scatter is not reduced by longer training.}
\label{fig:tt}
\end{figure}

The transverse traceless graviton on the ansatz of the Letter obeys the
massless minimally coupled scalar equation at zero spatial momentum.
It is dual to the stress tensor with $\Delta = 3$ in standard
quantization. Mass is exactly zero since the stress tensor is conserved.

On the lattice we use the bond anisotropy
\bbe
t(x) = \sigma(x)\sigma(x+\hat{e}_x) - \sigma(x)\sigma(x+\hat{e}_y),
\bbq
which projects onto the spin two representation and is traceless by
construction. We have measured $t$ on $10^4$ configurations at $L=128$.

The correlator is dominated by a contact term.
Writing $\langle tt \rangle(p) = c_0 + c_3 |p|^3 + \dots$, we find
$c_0 = 1.54$ and $c_3 = -0.057$ with a relative misfit of $0.015$.
The spin two signal is therefore present and is about four percent of the
measurement. We subtract $c_0$ before fitting so that the geometry is trained on the physical piece.

The fit does not converge to a useful geometry. The held out residual is $1.5 \times 10^{-2}$ across three seeds. This is two orders of magnitude above the scalar channels. The reconstructed metric functions grow without bound in the interior and the Einstein residuals are of order $10^2$. Thus we want to conclude that $32$ modes at zero spatial momentum can not able to constrain the
geometry at the available statistics.

We report this as a limitation. But there are two routes which can improve this. The shear sector at finite momentum supplies more independent data per
configuration and an improved lattice stress tensor with higher statistics would reduce the variance of the small $c_3$ piece. Thus a quantitative comparison with the bootstrap value $c_T/c_T^{\rm free} = 0.946538675(42)$ \cite{Chang:2024whx} remains open which can be a natural direction to follow in the future work.






%% =====================================================================
\section{Code and data availability}

In all simulations we use NumPy \cite{Harris:2020numpy} and PyTorch \cite{Paszke:2019pytorch} on CPU. The differentiable solver follows the neural differential equation approach of \cite{Chen:2018neuralode, Hashimoto:2020jug}.
Code and data are available from the author upon reasonable request.










\begin{thebibliography}{9}

\bibitem{Deng:2003wv}
Y.~Deng and H.~W.~J.~Bl\"ote,
Phys.\ Rev.\ E \textbf{68}, 036125 (2003),
\href{https://doi.org/10.1103/PhysRevE.68.036125}{doi:10.1103/PhysRevE.68.036125}.

\bibitem{Ferrenberg:2018zst}
A.~M.~Ferrenberg, J.~Xu, and D.~P.~Landau,
Phys.\ Rev.\ E \textbf{97}, 043301 (2018),
\href{https://doi.org/10.1103/PhysRevE.97.043301}{doi:10.1103/PhysRevE.97.043301}.

\bibitem{Wolff:1988uh}
U.~Wolff,
Phys.\ Rev.\ Lett.\ \textbf{62}, 361 (1989),
\href{https://doi.org/10.1103/PhysRevLett.62.361}{doi:10.1103/PhysRevLett.62.361}.

\bibitem{Chang:2024whx}
C.-H.~Chang \textit{et al.},
\href{https://arxiv.org/abs/2411.15300}{arXiv:2411.15300 [hep-th]}.

\bibitem{Hashimoto:2020jug}
K.~Hashimoto, H.-Y.~Hu, and Y.-Z.~You,
Mach.\ Learn.\ Sci.\ Tech.\ \textbf{2}, 035011 (2021),
\href{https://arxiv.org/abs/2006.00712}{arXiv:2006.00712 [hep-th]}.

\bibitem{Chen:2018neuralode}
R.~T.~Q.~Chen, Y.~Rubanova, J.~Bettencourt, and D.~Duvenaud,
in \textit{Advances in Neural Information Processing Systems 31}
(2018), p.~6571,
\href{https://arxiv.org/abs/1806.07366}{arXiv:1806.07366 [cs.LG]}.

\bibitem{Harris:2020numpy}
C.~R.~Harris \textit{et al.},
Nature \textbf{585}, 357 (2020),
\href{https://doi.org/10.1038/s41586-020-2649-2}
{doi:10.1038/s41586-020-2649-2}.

\bibitem{Paszke:2019pytorch}
A.~Paszke \textit{et al.},
in \textit{Advances in Neural Information Processing Systems 32}
(2019), p.~8024,
\href{https://arxiv.org/abs/1912.01703}{arXiv:1912.01703 [cs.LG]}.

\end{thebibliography}

\end{document}
